# Supplementary material for: How optical excitation controls the structure and properties of vanadium dioxide
Source: arXiv:1805.01430 ancillary file (2018-05-03)
Supplement: Supplementary file 1 [file sm.pdf]

# Supplemental material: How optical excitation controls the structure and properties of vanadium dioxide

Martin R. Otto,[1,*] Laurent P. René de Cotret,[1] David Valverde-Chavez,[1] Kunal L. Tiwari,[1] Nicolas Émond,[2] Mohamed Chaker,[2] David G. Cooke,[1] and Bradley J. Siwick[1,3,†]

[1]*Department of Physics, Center for the Physics of Materials, McGill University, 3600 University Street, Montreal, QC, CA*

[2]*Institut National de la Recherche Scientifique, Centre Énergie Matériaux et Télécommunications, Université du Québec, Varennes, Quebec J3X 1S2, Canada*

[3]*Department of Chemistry, McGill University, 801 Sherbrooke Street W, Montreal, QC, CA*

(Dated: May 3, 2018)

## CONTENTS

I. Ultrafast electron diffraction measurements (UED) 2

I.1. Experimental Setup 2

I.2. Peak dynamics analysis 3

I.3. Phase fraction analysis: model and estimation of $\Sigma_\chi$ 3

II. Time-resolved terahertz spectroscopy (TRTS) 5

II.1. Analysis and fitting example 5

II.2. Fluence dependence 5

II.3. Bruggeman effective medium theory 6

III. Real-space Structure Reconstruction 7

III.1. Intensity Extraction 7

III.2. Momentum-space cutoff 8

III.3. Patterson Pair-distribution Function 8

IV. Calculation of the electron temperature 10

V. DC sample characterization 10

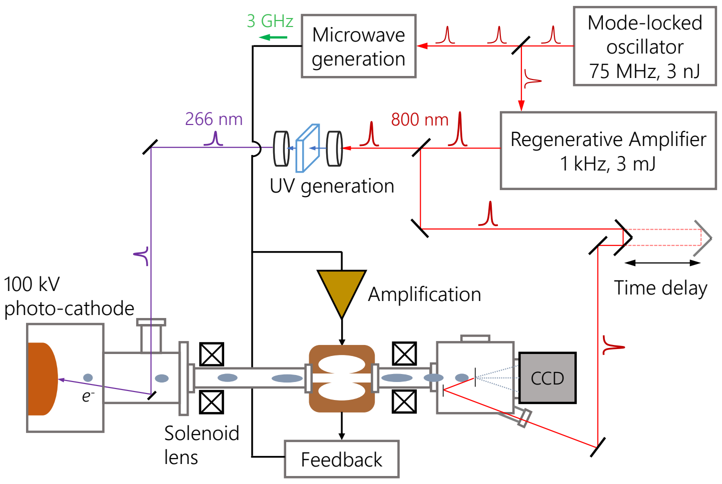


FIG. S1: Schematic of the ultrafast electron diffraction instrument with an RF-compressed source. The master laser system is a mode-locked Ti:sapphire oscillator which produced 3 nJ pulses at a repetition rate of ∼74.96 MHz. A synchronized ∼ 3 GHz harmonic tone is generated by direct photo-detection of the pulse train using a 12.5 GHz bandwidth diode as described in[S2]. The signal is amplified and drives the $TM_{010}$ mode of a single-cell compression cavity which is detuning-compensated continuously to ensure pulse arrival and compression stability. The oscillator pulse is amplified to 3mJ by a regenerative single-pass chirped pulsed amplified system which operates at 1 kHz. The output beam is split into two paths pump and probe, which are used for excitation of the sample and generation of UV and electrons respectively. Electrons are generated by photo-emission from a cathode and are accelerated to energies of ∼100 keV. Electrons scattered by the sample are collected and integrated by a charge-coupled-device (CCD) camera.

References 12

## I. ULTRAFAST ELECTRON DIFFRACTION MEASUREMENTS (UED)

### I.1. Experimental Setup

The ultrafast electron diffraction instrument is presented in Fig. S1 and described in complete detail in[S1,S2].

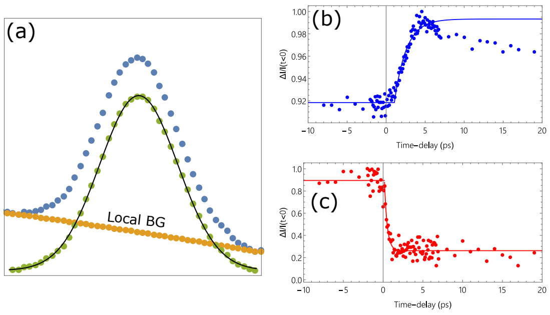


FIG. S2: (a) Example of fitting the (200) peak lineshape to Eqn. S1. The background is refined locally in the vicinity of the peak and subtracted in order to improve the fitting. (b) Example of the (200) peak dynamics and fitting at 30 mJ/cm$^2$. (c) Example of the (30$\bar{2}$) peak dynamics and fitting at 30 mJ/cm$^2$.

### I.2. Peak dynamics analysis

Images of the diffraction pattern collected by the CCD camera are azimuthally integrated and the time-dependent background of the entire pattern is removed using the dual-tree wavelet transform[S3]. For further analysis, a local background is estimated similarly in the vicinity of the peak of interest in order to correct for skewness as shown in FIG. S2 (a) for the (200) peak. At a given excitation fluence, the peak of interest at a time point $t$ is fit to a Gaussian function

$$I(s - s_0, t) = I_0(t)e^{-(s-s_0)^2/2\Gamma^2}, \tag{S1}$$

where $I_0(t)$ is the peak intensity, $s$ is the scattering vector, $s_0$ is the peak center and $\Gamma$ is the RMS peak width. The relative peak intensity is computed by finding the set of $I_0(t)$ for all pump probe time-delays. This data is then fit to $I(t, t_0) = \Theta(t - t_0)\Delta I_{(hkl)}\left(1 - e^{-(t-t_0)/\tau_{(hkl)}}\right)$ to extract the amplitude and time constants for each diffraction peak $(hkl)$ used in the analysis.

### I.3. Phase fraction analysis: model and estimation of $\Sigma_\chi$

The normalized relative intensity change $\tilde{i}(\mathcal{F})$ as a function of fluence $\mathcal{F}$ for the $\chi = (200)$ and (220) peaks can be written as

$$\begin{aligned}\tilde{i}(\mathcal{F}) &= \frac{\Delta I_\chi(\mathcal{F})}{\bar{I}_\chi^{M_1}} \\ &= \frac{\bar{I}_\chi^{M_1}F_{M_1}(\mathcal{F}) + \bar{I}_\chi^{R}F_R(\mathcal{F}) + \bar{I}_\chi^{\mathbb{M}}F_{\mathbb{M}}(\mathcal{F}) - \bar{I}_\chi^{M_1}}{\bar{I}_\chi^{M_1}}.\end{aligned} \tag{S2}$$

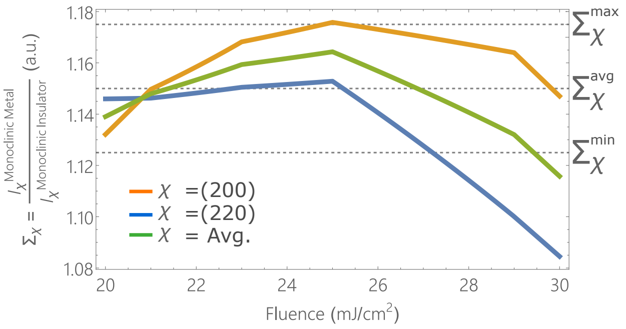


FIG. S3: Estimation of $\Sigma_\chi$ using ultrafast electron diffraction measurements and Eqn. S4. Peak intensity data $\Delta I(\mathcal{F})/\bar{I}_\chi^{M_1}$ for peaks $\chi = (200), (220)$ are used along with $\Delta I(\mathcal{F})/\bar{I}_{(30\bar{2})}^{M_1}$ in the high-fluence limit to solve for $\Sigma$. We assume that no $M_1$ crystallites remain $(1 = F_R + F_{\mathcal{M}})$. The orange (blue) curve is the calculation using the (200) ((220)) peak, and the green curve is the average, which is the final result we use under the assumption that $\Sigma_{(200)} = \Sigma_{(220)} = \Sigma$ is an intrinsic constant. $\Sigma_\chi^{\text{max}}$ is the maximum value (upper bound) determined using the data and $\Sigma_\chi^{\text{min}}$ is a lower bound enforced by the crystallite normalization condition $\sum_\phi F_\phi = 1$. $\Sigma_\chi^{\text{avg}}$ is the average of the green curve over the fluence range given by the bounds.

Equation (S2) includes intensity contributions $\bar{I}_\chi^\phi F_\phi$ from the three phases $\phi = M_1, \mathcal{M}, R$ of $VO_2$, where $F_\phi$ is the fluence-dependent volume phase fraction, and $\bar{I}_\chi^\phi$ is the peak intensity when *completely* in phase $\phi$. We may write it more compactly as

$$\tilde{i}(\mathcal{F}) = \frac{\Delta I_\chi}{\bar{I}_\chi^{M_1}} = \frac{1}{\bar{I}_\chi^{M_1}} \sum_{\phi = M_1, R, \mathcal{M}} \bar{I}_\chi^\phi F_\phi - 1. \tag{S3}$$

Using the condition that $\sum_\phi F_\phi = 1$ (crystallites are conserved) to eliminate $F_{M_1}$ we obtain

$$\frac{\Delta I_\chi}{\bar{I}_\chi^{M_1}} = (\Lambda_\chi - 1)\, F_R + (\Sigma_\chi - 1)\, F_{\mathcal{M}}, \tag{S4}$$

where $\Lambda_\chi = \bar{I}_\chi^R / \bar{I}_\chi^{M_1}$ and $\Sigma_\chi = \bar{I}_\chi^{\mathcal{M}} / \bar{I}_\chi^{M_1}$.$\Sigma_\chi$ can be determined in the high fluence limit by setting $F_{\mathcal{M}} \to 1 - F_R$ (*i.e.* there are no remaining $M_1$ crystallites in the sample at high fluences) and using $F_R = \Delta I_{(30\bar{2})}(\mathcal{F})/\bar{I}_{(30\bar{2})}^{M_1}$ involving the diffraction peak dynamics for the $30\bar{2}$ peak. The results for this estimation are shown in Fig. S3. We will assume that $\Sigma_{(200)} = \Sigma_{(220)} = \Sigma$. Consistency of the model requires that $\sum_\phi F_\phi = 1$ be respected, yielding a lower bound of $\Sigma^{\text{min}} = 1.125$. The maximum value we compute over the fluence range of 20 to 30 $\text{mJ/cm}^2$ is $\Sigma^{\text{max}} = 1.175$. Taking the average of the (200) and (220) results gives a value of $\Sigma = 1.150 \pm 0.025$.

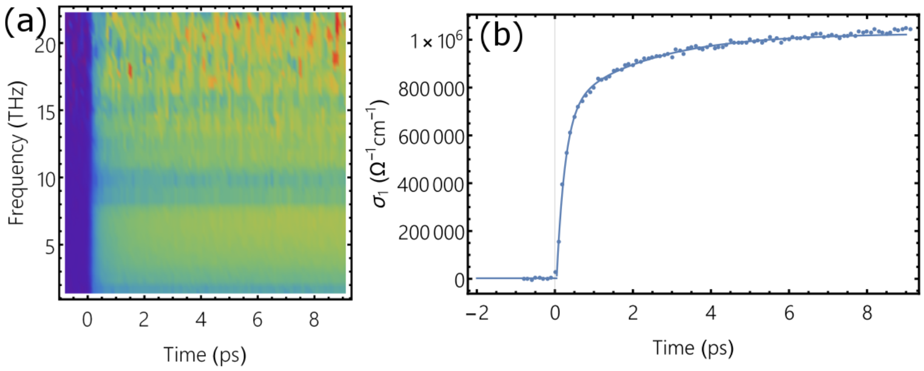


FIG. S4: (a) Real part of the terahertz conductivity $\sigma_1$ for frequencies up to 22 THz at 30 mJ/cm$^2$. (b) Real component of the terahertz conductivity response $\sigma_1$ shown in (a) integrated from 2-6 THz. The solid line is a fit to the bi-exponential function expressed in Eqn. S5.

## II. TIME-RESOLVED TERAHERTZ SPECTROSCOPY (TRTS)

### II.1. Analysis and fitting example

The terahertz conductivity $\sigma(\omega) = \sigma_1(\omega) + i\sigma_2(\omega)$ is computed from the real and imaginary $E-$field components obtained by the spectrometer. A typical broadband pump-probe measurement of $\sigma_1$ is shown in Fig. S4 (a). The THz conductivity response is integrated from $\omega_1/2\pi = 2$ to $\omega_2/2\pi = 6$ THz and the data is fit to a bi-exponential of the form

$$\sigma_1(t,t_0) = \int_{\omega_1}^{\omega_2} \Re\left\{\sigma(\omega;t,t_0)\right\} \mathrm{d}\omega,$$

$$\sigma_1(t,t_0) = \Theta\left(t-t_0\right)\Delta\sigma_1^{\text{fast}}\left(1-e^{-(t-t_0)/\tau_{\text{fast}}}\right)+\cdots$$
$$+\,\Theta\left(t-t_0\right)\Delta\sigma_1^{\text{slow}}\left(1-e^{-(t-t_0)/\tau_{\text{slow}}}\right), \tag{S5}$$

where $t_0$ is "time-zero", $\Delta\sigma_1^{\text{fast}}$ and $\Delta\sigma_1^{\text{slow}}$ are the amplitudes of the fast and slow conductivity components respectively, which in turn have time constants $\tau_{\text{fast}}$ and $\tau_{\text{slow}}$. An example of the fitting for data at a fluene of 30 mJ/cm$^2$ is shown in Fig. S4 (b).

### II.2. Fluence dependence

The TRTS measurements are performed at different fluences which are all shown in Fig. S6 in normalized form for clarity. The character of the fluence dependence of $\tau_{\text{slow}}$ is clearly visible, showing a decreasing time constant at higher fluence. The Amplitudes $\Delta\sigma_1^{\text{fast}}$ and $\Delta\sigma_1^{\text{slow}}$ are shown in Fig. 4 (b) of the main text and the time constants $\tau_{\text{fast}}$ and $\tau_{\text{slow}}$ are shown in Fig. 5 of the main text.

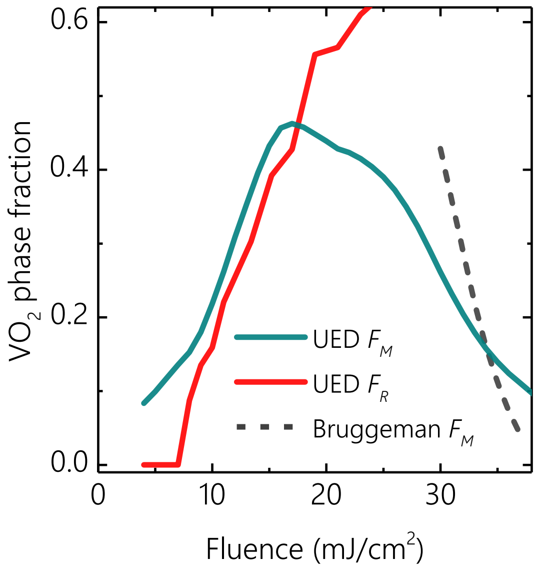


FIG. S5: Comparison of the phase fractional models: Red and cyan lines are calculations of $F_R$ and $F_{\mathcal{M}}$ using the UED measurements and (S4) (Also shown in FIG. 4 (b) of the main text). The dashed gray line is computed from the TRTS measurements (FIG. 4 (c) of main text) using (S6).

### II.3. Bruggeman effective medium theory

The TRTS measurements by be analyzed in a similar manner using a Bruggeman effective medium model[S4] in the limit where the material is mostly metallic ($F_{\mathcal{M}} + F_R \to 1$). The conductivities determined from the TRTS measurements presented in FIG. 4 (c) of the main text. $\Delta\sigma_1^{\text{fast}}$ and $\Delta\sigma_1^{\text{slow}}$ form two contributions to the an effective medium for which the Bruggeman model states

$$F_R \frac{\Delta\sigma_1^{\text{fast}} - \sigma_e}{\Delta\sigma_1^{\text{fast}} + 2\sigma_e} + F_{\mathcal{M}} \frac{\Delta\sigma_1^{\text{slow}} - \sigma_e}{\Delta\sigma_1^{\text{slow}} + 2\sigma_e} = 0, \tag{S6}$$

where $\sigma_e$ is an *effective* conductivity of the heterogeneous material. Due to the time-resolution provided by the TRTS data, we have access to all conductivity terms, since we temporally distinguish between $\sigma_1^{\text{fast}}$ and $\sigma_1^{\text{slow}}$, and $\sigma_e$ is the total measured conductivity (after 10 ps). In the high-fluence limit, we use (S6) to compute $F_{\mathcal{M}}$ which is shown in FIG. S5. We find that this yields a result consistent with what was determined using the UED measurements.

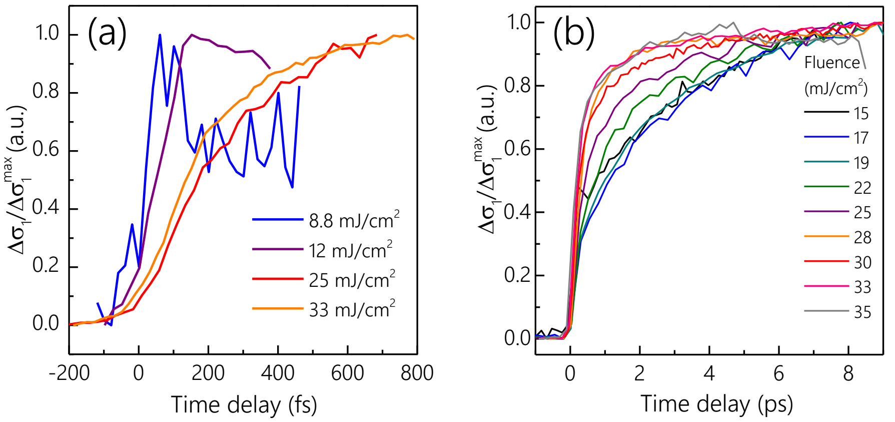


FIG. S6: Time-resolved terahertz spectroscopy measurements of normalized $\Delta\sigma_1$ for various fluences. The conductivity response is integrated from 2-6 THz. (a) Initial conductivity response of the $VO_2$ film within 1 ps. At lower fluences, an extremely fast, pulse-limited transient metalization is observed and originated from carrier excitation. (b) Conductivity response within the first 10 ps following photo-excitation, illustrating the fluence dependence.

## III. REAL-SPACE STRUCTURE RECONSTRUCTION

$\Phi(\boldsymbol{x})$, the real-space electrostatic potential, is given by an inverse Fourier-transform of the structure factors:

$$\Phi(\boldsymbol{x}) = \sum_{\{\boldsymbol{G}\}} \sqrt{I_{\boldsymbol{G}}} \exp\left(i\varphi_{\boldsymbol{G}}\right) \cos(\boldsymbol{x} \cdot \boldsymbol{G}), \tag{S7}$$

where the set $\{\boldsymbol{G}\}$ is understood to be the set of scattering vectors $\boldsymbol{G}_{hkl} = h\boldsymbol{b}_1 + k\boldsymbol{b}_2 + l\boldsymbol{b}_3$ lying within range of angles visible to the diffractometer, $I_{\boldsymbol{G}}$ is the diffraction intensity associated *only* with scattering vector $\boldsymbol{G}$, and $\phi(\boldsymbol{G})$ is the diffraction phase.

Diffraction measurements are not sensitive to the phases $\phi(\boldsymbol{G})$. We use the centro-symmetry of $VO_2$ rutile and monoclinic M1 phases (and hence the monoclinic metal phase), which limits the phases to $\{0, \pi\}$. Then, we can infer the phases from the well-known crystal structures.

### III.1. Intensity Extraction

The extraction of diffraction intensity associated with a reflection $\boldsymbol{G} = (hkl)$ is arduous for the case of $VO_2$ because of overlapping reflections. Since reflections most often overlap by more than 50% of their full-width at half-max (FWHM), Le Bail intensity decomposition (iterative or

otherwise) was not successful. We instead opted to distribute intensities proportionally according to a model structure, which is well-known in the case of $VO_2$. For an experimental diffraction pattern $I_{\text{exp}}(q)$, we extract the diffracted intensity associated only with the reflection $\boldsymbol{G}$, $I_{\boldsymbol{G}}$ like so:

$$I_{\boldsymbol{G}} = I_{\text{exp}}(|\boldsymbol{G}|) \times \frac{S(\boldsymbol{G})^2}{I_{\text{theo}}(|\boldsymbol{G}|)} \tag{S8}$$

where $I_{\text{theo}}$ is a simulated electron powder diffraction pattern, and $S(\boldsymbol{G})$ is the theoretical structure factor associated with reflection $\boldsymbol{G}$. The calculation of theoretical quantities are provided by the open-source package scikit-ued[S5]

### III.2. Momentum-space cutoff

Dynamics in the electron diffraction pattern are not present at all scattering vectors; therefore, changes in the electrostatic potential (which highlights the Monoclinic metal structure) can be affected by noise in the high scattering vector regions. Figure S7 shows multiple versions of Figure 3 with different scattering vector cutoffs used in the reconstruction of the electrostatic potential change.

The salient features of Figure 3 are not affected by the cutoff scattering vector beyond an expected broadening (a cutoff in reciprocal space is equivalent to a low-pass filter).

### III.3. Patterson Pair-distribution Function

The reconstruction of real-space electrostatic potential from diffraction data requires the knowledge of diffraction phases as well, information that is not available to ultrafast electron diffraction measurements. We get around this by using the known crystal structures of monoclinic $M_1$ and rutile $VO_2$. Note that the crystal structure of the $\mathcal{M}$ phase is identical to the monoclinic $M_1$ phase.

To validate the use of theoretical diffraction phases in the reconstructed electrostatic potential maps, we calculate the Patterson radial pair-distribution function $G(r,t)$ in two ways:

- Directly from the polycrystalline diffraction patterns;
- As the autocorrelation of the 3D electrostatic potential.

To calculate the Patterson radial pair-distribution function, the diffracted intensity $I(q,t)$ must be normalized. The normalized (or reduced) intensity $\mathcal{I}$ is defined for a general unit cell $U$ of $N$

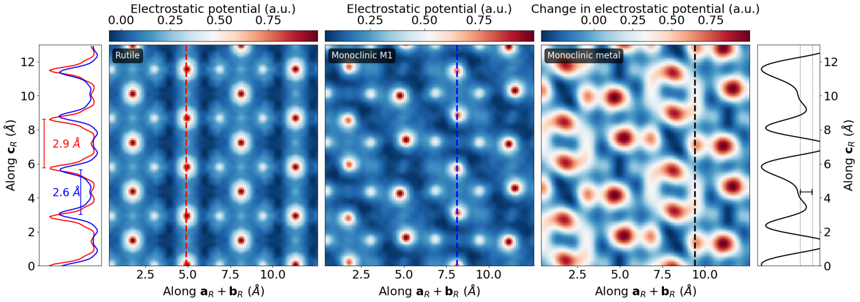


(a) Electrostatic potential map of $VO_2$. The Monoclinic metal map is rendered with $s < 0.4$ Å$^{-1}$

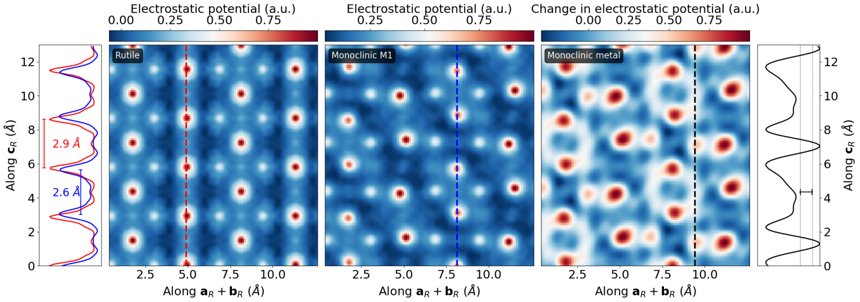


(b) Electrostatic potential map of $VO_2$. The Monoclinic metal map is rendered with $s < 0.5$ Å$^{-1}$. This is the cutoff used in Figure 3.

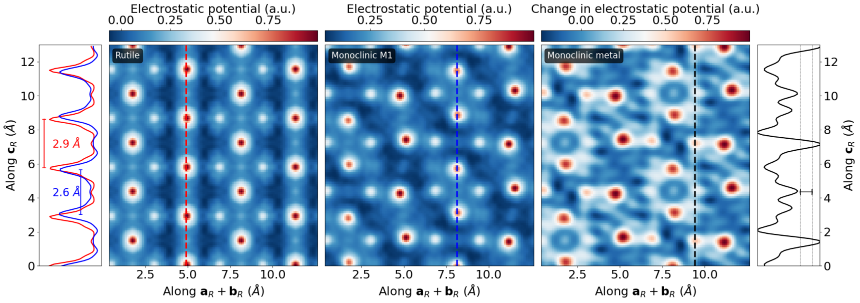


(c) Electrostatic potential map of $VO_2$. The Monoclinic metal map is rendered with $s < 0.6$ Å$^{-1}$

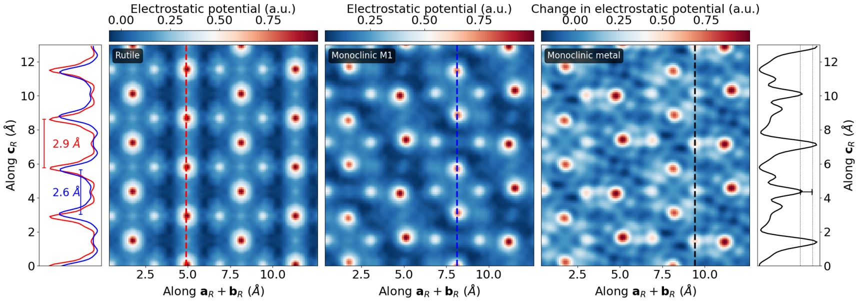


(d) Electrostatic potential map of $VO_2$. The Monoclinic metal map is rendered with $s < 0.7$ Å$^{-1}$

FIG. S7: Atominc potential maps for various scattering vector cut-offs.

atoms ($a$) as follows:

$$\mathcal{I}(q,t) \equiv I(q,t) - \frac{1}{N}\sum_{a\in U}^{N} |f_a(q)|^2 \Bigg/ \frac{1}{N}\sum_{a\in U}^{N} |f_a(q)|^2 \tag{S9}$$

where $f_a(q)$ is understood to be the atomic form factor for electrons for atom $a$. The Patterson radial pair-distribution function is then given by:

$$G(r,t) = \frac{1}{2\pi^2 r}\int_0^\infty \mathrm{d}q\; q\; \sin(r\cdot q)\; \mathcal{I}(q,t) \tag{S10}$$

as per Fultz and Howe[S6].

The radial pair-distribution function can also be computed as the radial autocorrelation of a 3D electrostatic potential $\Phi(r(x,y,z),t)$:

$$G(r,t) = \int \mathrm{d}S_r\; \Phi(r,t) * \Phi(r,t) \tag{S11}$$

where $\mathrm{d}S_r$ is the spherical surface element, and ($*$) is understood to be the correlation operator.

The radial pair-distribution function of the un-pumped monoclinic $M_1$ $VO_2$, $G(r, t < 0)$, is presented in fig. S8. It is contrasted with the radial autocorrelation of an electrostatic potential volume of $2\times2\times2$ unit cells of monoclinic $M_1$ $VO_2$. The agreement between the two curves is close to perfect, indicating that the use of theoretical diffraction phases in this work is fully consistent with other analyses based on the diffraction data.

## IV. CALCULATION OF THE ELECTRON TEMPERATURE

We follow the prescription shown in Tomlin[S7]. The 50 nm thick $VO_2$ sample is on top of a 40 nm $SiN_x$ substrate which is illuminated by a beam with fluence $\mathcal{F}$ (normal incidence is assumed). The complex index of refraction for $VO_2$ is $\tilde{n} = 2.9 + i0.5$[S8,S9] and $n = 2.0$ for $SiN_x$. We determine the absorption to be $\mathcal{A} = 0.222$ at 800 nm. $VO_2$ has a unit cell volume of $V_{\text{unit-cell}} = 117$ Å$^3$ and the number of unit cells in the sample is $N = V_{\text{sample}}/V_{\text{unit-cell}}$. The energy deposited per unit cell is given by

$$\varepsilon(\mathcal{F}) = \frac{\mathcal{A}}{N}\mathcal{F}\; A_{\text{sample}}, \tag{S12}$$

where $A_{\text{sample}}$ is the area of the sample on the substrate (250 $\mu$m by 250 $\mu$m).

## V. DC SAMPLE CHARACTERIZATION

The DC properties of the $VO_2$ films grown by pulsed laser deposition are characterized following growth of the films. Details of the deposition recipe are presented in Hendaoui et al.[S10]. The results

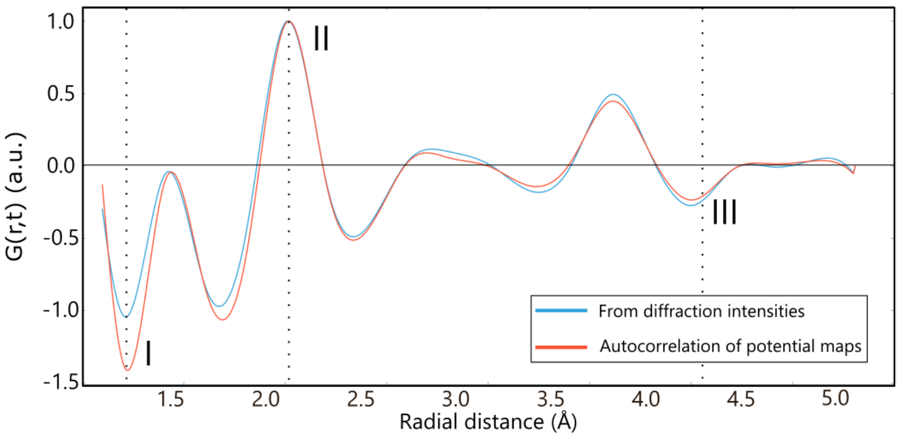


FIG. S8: Comparison of the radial pair-distribution function computed in two separate ways from static diffraction of monoclinic M1 $VO_2$. The blue curve has been calculated directly from the polycrystalline diffraction intensity. The orange curve was calculated by reconstructing a large real-space electrostatic potential map (2x2x2 unit cells) and autocorrelating it. Negative feature at I is due to the average half V-V dimer length. Positive feature at II is due to the average V-O distance around the octahedron. Negative feature at III represents the sum of dimerized and undimerized average V-V distance.

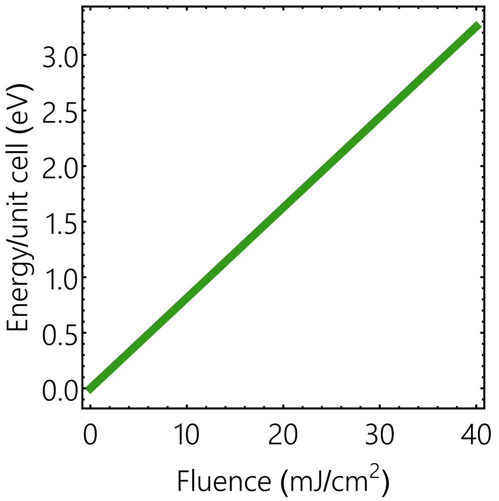


FIG. S9: Calculated absorbed energy per unit cell $\epsilon$ as a function of fluence for a 50 nm thick $VO_2$ film on a 40 nm $SiN_x$ substrate. The area of the sample window is 250 $\mu$m by 250 $\mu$m.

for the 4-point resistivity are shown in FIG. S10 (a) and (b).

A 50 nm thick spectator $VO_2$ sample was also produced alongside the other samples for X-ray diffraction (XRD) characterization. The XRD trace for the 50 nm $VO_2$ film in shown in S10 (c) with a reference film to identify the relevant peaks.

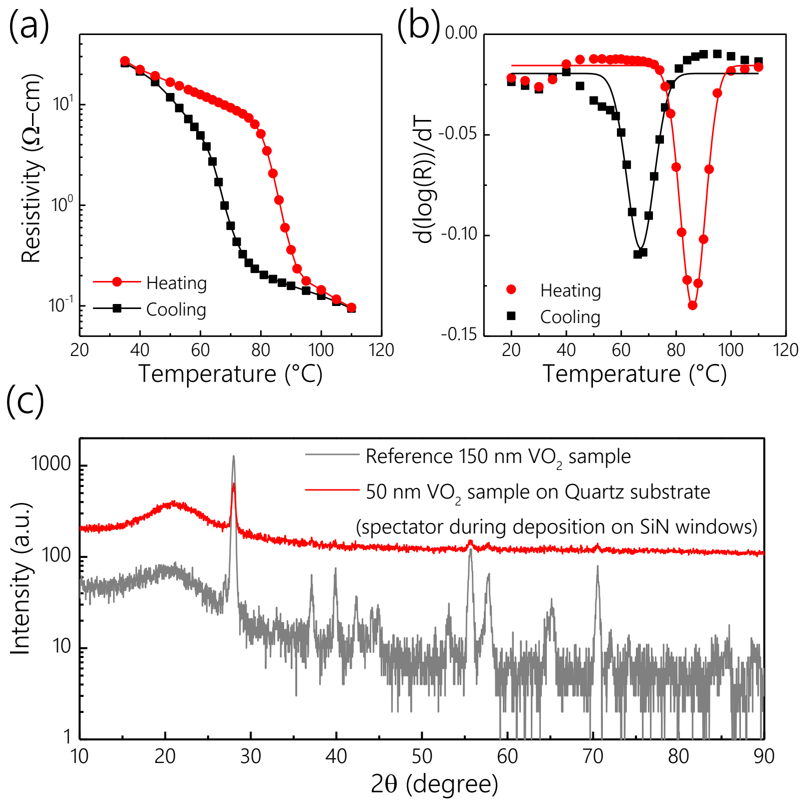


FIG. S10: Characterization data for the $VO_2$ films. (a) DC 4-point resistivity $R$ measurement performed during heating (red circles) followed by cooling (black squares) to show the expected IMT and hysteresis character. (b) Plot of $\frac{d}{dT}\ln(R)$ vs. temperature $T$.


* martin.otto@mail.mcgill.ca

† bradley.siwick@mcgill.ca



[S1] R. P. Chatelain, V. R. Morrison, C. Godbout, and B. J. Siwick, Applied Physics Letters **101**, 081901 (2012), ISSN 00036951, URL http://link.aip.org/link/APPLAB/v101/i8/p081901/s1&Agg=doi.

[S2] M. R. Otto, L. P. R. de Cotret, M. J. Stern, and B. J. Siwick, Structural Dynamics **4**, 051101 (2017), https://doi.org/10.1063/1.4989960, URL https://doi.org/10.1063/1.4989960.

[S3] L. P. René de Cotret and B. J. Siwick, Structural Dynamics **4**, 044004 (2017), https://doi.org/10.1063/1.4972518, URL https://doi.org/10.1063/1.4972518.

[S4] R. Landauer, AIP Conference Proceedings **40**, 2 (1978), https://aip.scitation.org/doi/pdf/10.1063/1.31150, URL https://aip.scitation.org/doi/abs/10.1063/1.31150.

[S5] L. P. René de Cotret, scikit-ued : open-source collection of algorithms and routines for (ultrafast) electron diffraction, https://github.com/LaurentRDC/scikit-ued, accessed: 2018-03-19.

[S6] B. Fultz and J. M. Howe, Transmission electron microscopy and diffractometry of materials (Google eBook)

(Springer, 2002), ISBN 3540437649, URL http://books.google.com/books?id=LjrJ59378EcC&pgis=1.

[S7] S. G. Tomlin, Journal of Physics D: Applied Physics **1**, 1667 (1968), URL http://stacks.iop.org/0022-3727/1/i=12/a=312.

[S8] A. Cavalleri, C. Tóth, C. W. Siders, J. A. Squier, F. Ráksi, P. Forget, and J. C. Kieffer, Phys. Rev. Lett. **87**, 237401 (2001), URL https://link.aps.org/doi/10.1103/PhysRevLett.87.237401.

[S9] Z. He and A. J. Millis, Phys. Rev. B **93**, 115126 (2016), URL https://link.aps.org/doi/10.1103/PhysRevB.93.115126.

[S10] A. Hendaoui, N. Émond, M. Chaker, and Émile Haddad, Applied Physics Letters **102**, 061107 (2013), https://doi.org/10.1063/1.4792277, URL https://doi.org/10.1063/1.4792277.
